# Supplementary material for: NSA: Neuro-symbolic ARC Challenge
Source: arXiv:2501.04424 source file (2025-01-08)
Supplement: Supplementary file 1 [file appendix.tex]

\clearpage
\setcounter{page}{1}
\maketitlesupplementary

\section{Appendix}
\label{sec:appendix}
